# Supplementary material for: Neighborhood Commonality-aware Evolution Network for Continuous Generalized Category Discovery
Source: arXiv:2412.05573 source file (2024-12-07)
Supplement: Supplementary file 1 [file supp.tex]

\section{Losses}

\begin{table}[ht]\small
    \begin{center}
    \begin{tabular}{c|c|ccc|ccc}
    \toprule
       \multirow{2}{*}{Exp.} &  \multirow{2}{*}{Method}  & \multicolumn{3}{c|}{CUB200} & \multicolumn{3}{c}{CIFAR100} \\
    \cmidrule{3-8}
         {} & {}    & {All} & {Old} & {New}  & {All} & {Old} & {New}\\
    \midrule
         {1)} & {w/o $\mathcal{L}_{\text{crl}}$}     & {55.0}  & {46.2} & {59.0} & {74.6}  & {77.4} & {69.0} \\
         {2)} & {w/o $\mathcal{L}_{\text{cru}}$}     & {60.0}  & {59.3} & {60.3} & {58.1}  & {69.8} & {34.2} \\
         {3)} & {w/o $\mathcal{L}_{\text{sup}}$}     & {60.1}  & {55.3} & {62.5} & {72.4}  & {75.2} & {66.8} \\
         {4)} & {w/o $\mathcal{L}_{\text{unsup}}$}   & {63.1}  & {61.7} & {63.8} & {79.7}  & {80.8} & \textbf{77.5} \\
    \midrule
         {5)} & {w all}                              & \textbf{67.4}  & \textbf{69.2} & \textbf{66.5} & \textbf{80.0}  & \textbf{81.7} & {76.3} \\
    \bottomrule
    \end{tabular}
    \caption{Ablation studies on losses.}
    \label{tab:ablat_losses}
    \end{center}
\end{table}

To investigate the influence of each loss used in our proposed PNP, we remove each loss individually and compare the corresponding clustering accuracy with that given by using all losses. As shown in \cref{tab:ablat_losses}, removing each loss drops the clustering accuracy indicating that each loss is important for PNP. Further, comparing the clustering accuracy given by removing other losses, removing $\mathcal{L}_{\text{crl}}$ drops the clustering accuracy by a relatively larger margin on CUB200. Conversely, removing $\mathcal{L}_{\text{cru}}$ results in a larger drop in the clustering accuracy compared to that given by removing other losses on CIFAR100. The reason may stem from that CUB200 is a fine-grained dataset that needs stronger supervision compared to the coarse-grained dataset CIFAR100 to split each class well.

\section{Trainable \textit{VS} Frozen}
\begin{table}[h]
    \centering
    \begin{tabular}{l|cccc}
    \toprule
        Method & {$K^e$} & All & Old & New \\
    \midrule
        w/o PP         &  175 & 62.4 & 59.1 & 64.1 \\ 
        Frozen  PP     &  183 & 66.4 & 65.6 & 66.9 \\
        Trainable PP   &  183 & 67.4 & 69.2 & 66.5 \\
    \bottomrule
    \end{tabular}
    \caption{Estimated category number and clustering accuracy of different settings, where PP refers to the potential prototypes. }
    \label{tab:fvt}
\end{table}

\begin{table*}[ht]\small
    \centering
    \begin{tabular}{c|c|ccc|ccc|ccc|ccc}
    \toprule
    \multirow{2}{*}{Methods}& \multirow{2}{*}{Known $K^u$} & \multicolumn{3}{c|}{CUB200} & \multicolumn{3}{c|}{Stanford Cars} & \multicolumn{3}{c}{FGVC-Aircraft} & \multicolumn{3}{c}{Oxford-Pet}\\
    \cmidrule(r){3-5}  \cmidrule(r){6-8} \cmidrule(r){9-11} \cmidrule(r){12-14}
    {} & {} & {All} & {Old} & {New}  & {All} & {Old} & {New} & {All} & {Old} & {New} & {All} & {Old} & {New} \\
    \midrule
         k-means~\cite{macqueen1967some}    & \ding{51}  & 34.3 & 38.9 & 32.1 & 12.8 & 10.6 & 13.8 & 16.0 & 14.4 & 16.8 & {77.1}  & {70.1} & {80.7} \\
         RS+~\cite{han2021autonovel}        & \ding{51}  & 33.3 & 51.6 & 24.2 & 28.3 & 61.8 & 12.1 & 26.9 & 36.4 & 22.2 & {-}  & {-} & {-}\\
         UNO+~\cite{fini2021unified}        & \ding{51}  & 35.1 & 49.0 & 28.1 & 35.5 & 70.5 & 18.6 & 40.3 & 56.4 & 32.2 & {-}  & {-} & {-} \\    
         ORCA~\cite{cao2021openworld}       & \ding{51}  & 35.3 & 45.6 & 30.2 & 23.5 & 50.1 & 10.7 & 22.0 & 31.8 & 17.1 & {-}  & {-} & {-} \\
         GCD~\cite{vaze2022generalized}     & \ding{51}  & 51.3 & 56.6 & 48.7 & 39.0 & 57.6 & 29.9 & 45.0 & 41.1 & 46.9 & {-}  & {-} & {-}\\
         CiPR~\cite{hao2024cipr}            & \ding{51}  & 57.1 & 58.7 & 55.6 & 47.0 & 61.5 & 40.1 & {-}  & {-} & {-} & {-}  & {-} & {-} \\ 
         SimGCD~\cite{wen2023parametric}    & \ding{51}  & 60.3 & 65.6 & 57.7 & 53.8 & 71.9 & 45.0 & 54.2 & 59.1 & 51.8 & {-}  & {-} & {-} \\
         PromptCAL~\cite{zhang2023promptcal}& \ding{51}  & 62.9 & 64.4 & 62.1 & 50.2 & 70.1 & 40.6 & 52.2 & 52.2 & 52.3 & {-}  & {-} & {-} \\
         $\mu$GCD~\cite{vaze2023no}         & \ding{51}  & 65.7 & 68.0 & {64.6} & {56.5} & 68.1 & \textbf{50.9} & 53.8 & 55.4 & {53.0} & {-}  & {-} & {-} \\
         SPTNet~\cite{wang2024sptnet} & \ding{51}  & 65.8 & 68.8 & {65.1} & \textbf{59.0} & \textbf{79.2} & 49.3 & \textbf{59.3} & 61.8 & \textbf{58.1} & {-}  & {-} & {-}\\
         InfoSieve~\cite{rastegar2023learn} & \ding{51}  & \textbf{69.4} & \textbf{77.9} & \textbf{65.2} & {55.7} & {74.8} & 46.4 & {56.3} & \textbf{63.7} & 52.5 & \textbf{91.8}  & \textbf{92.6} & \textbf{91.3}\\

         \midrule
         GCD$^*$~\cite{vaze2022generalized} & \ding{55}   & 47.1 & 55.1 & 44.8 & 35.0 & 56.0 & 24.8 & 40.1 & 40.8 & 42.8 & {80.2}  & {85.1} & {77.6} \\
         Yang \etal~\cite{yang2023generalized} & \ding{55}& 58.0 & 65.0 & 43.9 & 47.6 & \textbf{70.6} & 33.8 & {-}  & {-} & {-} & {-}  & {-} & {-}\\ 
         GPC~\cite{zhao2023learning}        & \ding{55}   & 52.0 & 55.5 & 47.5 & 38.2 & 58.9 & 27.4 & 43.3 & 40.7 & 44.8 & {-}  & {-} & {-}\\
         % SimGCD$^*$~\cite{wen2023parametric}& \ding{55}   & 61.5 & 66.4 & 59.1 & 49.1 & 65.1 & 41.3 & 43.7 & 33.1 & \textbf{47.1} & 89.5 & 86.5 & \textbf{91.1} \\
         DCCL$^*$~\cite{pu2023dynamic}      & \ding{55}   & 63.5 & 60.8 & 64.9 & 43.1 & 55.7 & 36.2 & 42.7 & 41.5 & 43.4 & {88.1}  & \textbf{88.2} & {88.0}\\
    % \midrule
    
         PNP(Ours)        & \ding{55} & \textbf{67.4} & \textbf{69.2} & \textbf{66.5} & \textbf{57.3} & {70.2} & \textbf{51.1} & \textbf{47.0} & \textbf{49.5} & {45.7} & \textbf{89.7}  & {87.6} & \textbf{90.8}\\
         
   \bottomrule  
    \end{tabular}
    \caption{Results on the Semantic Shift Benchmark, where $^*$ denotes our reproduced results or from their publicly available results, $-$ denotes no results reported in the corresponding works, and best results with/without taking the category number $K^u$ as the prior are highlighted in bold font.}
    \label{tab:ssb_new}
\end{table*}

% \vspace{-0.5cm}

\begin{table*}[ht]\small
    \centering
    \begin{tabular}{c|c|ccc|ccc|ccc|ccc}
    \toprule
    \multirow{2}{*}{Methods}& \multirow{2}{*}{Known $K^u$} & \multicolumn{3}{c|}{CIFAR10} & \multicolumn{3}{c|}{CIFAR100} & \multicolumn{3}{c|}{ImageNet100} & \multicolumn{3}{c}{Herbarium 19} \\
    \cmidrule(r){3-5}  \cmidrule(r){6-8} \cmidrule(r){9-11} \cmidrule(r){12-14}
    {} & {} & {All} & {Old} & {New}  & {All} & {Old} & {New} & {All} & {Old} & {New} & {All} & {Old} & {New} \\
    \midrule
         k-means~\cite{macqueen1967some}    & \ding{51} & 83.6 & 85.7 & 82.5 & 52.0 & 52.2 & 50.8 & 72.7 & 75.5 & 71.3 & 13.0 & 12.2 & 13.4 \\
         RankStats+~\cite{han2021autonovel} & \ding{51} & 46.8 & 19.2 & 60.5 & 58.2 & 77.6 & 19.3 & 37.1 & 61.6 & 24.8 & 27.9 & 55.8 & 12.8 \\
         UNO+~\cite{fini2021unified}        & \ding{51} & 68.6 & 98.3 & 53.8 & 69.5 & 80.6 & 47.2 & 70.3 & 95.0 & 57.9 & 28.3 & 53.7 & 14.7 \\   
         ORCA~\cite{cao2021openworld}       & \ding{51} & 81.8 & 86.2 & 79.6 & 69.0 & 77.4 & 52.0 & 73.5 & 92.6 & 63.9 & 20.9 & 30.9 & 15.5 \\
         GCD~\cite{vaze2022generalized}     & \ding{51} & 91.5 & \textbf{97.9} & 88.2 & 73.0 & 76.2 & 66.5 & {72.7}  & {91.8} & {63.8} & 35.4 & 51.0 & 27.0 \\
         SimGCD~\cite{wen2023parametric}    & \ding{51}  & 97.1 & 95.1 & {98.1} & 80.1 & 81.2 & {77.8} & {83.0} & {93.1} & {77.9} & \textbf{44.0} & 58.0 & \textbf{36.4} \\
         InfoSieve~\cite{rastegar2023learn} & \ding{51}  & 94.8 & 97.7 & 93.4  & 78.3 & 82.2 & 70.5 & {80.5} & {93.8} & {73.8} & 41.0 & \textbf{55.4} & 33.2 \\
         CiPR~\cite{hao2024cipr}            & \ding{51}  & 97.7 & 97.5 & 97.7 & \textbf{81.5} & 82.4 & \textbf{79.7} & 80.5 & 84.9 & 78.3 & 36.8 & 45.4 & 32.6\\
         SPTNet~\cite{wang2024sptnet} & \ding{51}  & 97.3 & 95.0 & \textbf{98.6} & 81.3 & \textbf{84.3} & 75.6 & \textbf{85.4} & \textbf{93.2} & \textbf{81.4} & 43.4 & 58.7 & 35.2 \\
         PromptCAL~\cite{zhang2023promptcal}& \ding{51}  & \textbf{97.9} & {96.6} & {98.5} & {81.2} & {84.2} & 75.3 & {83.1} & {92.7} & {78.3} & - & - & - \\

         \midrule
         % SimGCD$^*$~\cite{wen2023parametric}& \ding{55}   & 82.9 & 96.3 & 76.2 & \textbf{80.1} & 81.2 & \textbf{77.8} & 81.7 & 91.2 & 76.8 & 39.7 & \textbf{58.2} & 29.7 \\
         GCD$^*$~\cite{vaze2022generalized}& \ding{55}   & 88.6 & 96.2 & 84.9 & 73.0 & 76.2 & 66.5 & {72.7} & {91.8} & {63.8} & 30.9 & 36.3 & 28.0 \\
         GPC~\cite{zhao2023learning}       & \ding{55}   & 90.6 & \textbf{97.6} & 87.0 & 75.4 & \textbf{84.6} & 60.1 & {75.3} & \textbf{93.4} & {66.7} & 36.5 & 51.7 & 27.9 \\
         Yang \etal~\cite{yang2023generalized} & \ding{55}& 92.3 & 91.4 & 94.4 & 78.5 & 81.4 & 75.6 & 81.1 & 80.3 & \textbf{81.8} & 36.3 & 53.1 & 30.7 \\
         DCCL$^*$~\cite{pu2023dynamic}     & \ding{55}   & \textbf{96.3} & {96.5} & \textbf{96.9} & 75.3 & 76.8 & 70.2 & {80.5} & {90.5} & {76.2} & 39.8 & 50.5 & \textbf{34.1} \\
         PNP(Ours)                         & \ding{55}   & {90.2} & {95.0} & {87.8} & \textbf{80.0} & {80.7} & \textbf{76.3} & \textbf{82.4} & {92.9} & {77.2} & \textbf{41.1} & \textbf{56.2} & {32.9} \\
         
   \bottomrule  
    \end{tabular}
    \caption{Results on generic image recognition datasets and more challenging fine-grained and long-tailed datasets, where $^*$ denotes our reproduced results or from their publicly available results. Best results with/without taking the category number $K^u$ as the prior are highlighted in bold font. }
    \label{tab:cch_new}
\end{table*}

\begin{table*}[ht]\small
    \centering
    \begin{tabular}{c|c|ccc|ccc|ccc|ccc}
    \toprule
    \multirow{2}{*}{Methods}& \multirow{2}{*}{Known $K^u$} & \multicolumn{3}{c|}{Herbarium 19} & \multicolumn{3}{c|}{Stanford Cars} & \multicolumn{3}{c}{FGVC-Aircraft} & \multicolumn{3}{c}{CIFAR10}\\
    \cmidrule(r){3-5}  \cmidrule(r){6-8} \cmidrule(r){9-11} \cmidrule(r){12-14}
    {} & {} & {All} & {Old} & {New}  & {All} & {Old} & {New} & {All} & {Old} & {New} & {All} & {Old} & {New} \\
    \midrule
         % GCD~\cite{vaze2022generalized}     & \ding{51}  & 51.3 & 56.6 & 48.7 & 39.0 & 57.6 & 29.9 & 45.0 & 41.1 & 46.9 & {-}  & {-} & {-}\\
         SimGCD~\cite{wen2023parametric}     & \ding{51}  & 44.0 & 58.0 & 36.4 & 53.8 & 71.9 & 45.0 & 54.2 & 59.1 & 51.8 & 97.1 & 95.1 & 98.1 \\
         SimGCD$^*$~\cite{wen2023parametric} & \ding{55}  & 39.7 & 58.2 & 29.7 & 49.1 & 65.1 & 41.3 & 43.7 & 33.1 & 47.1 & 89.5 & 86.5 & 91.1 \\

         PNP(Ours)                           & \ding{55}  & 41.1 & 56.2 & 32.9 & 57.3 & 70.2 & 51.1 & 47.0 & 49.5 & 45.7 & 90.2 & 95.0 & 87.8\\
         
   \bottomrule  
    \end{tabular}
    \caption{Clustering accuracy of SimGCD and our proposed PNP, where $^*$ denotes our reproduced results.}
    \label{tab:ssb_new_new}
\end{table*}

Table \ref{tab:fvt} shows the estimated category number and clustering accuracy given by removing potential prototypes (PP), freezing PP, and setting PP trainable, respectively. We can see that compared to the performance given by removing PP, using frozen PP or trainable PP both increases the estimated category number and improves the clustering accuracy. The results further validate that using PP helps discover more novel classes. Compared to the clustering accuracy given by using frozen PP, though using trainable PP drops the performance on ``NEW'' classes slightly, it improves the performance on ``OLD'' classes by a relatively larger margin. This indicates that using trainable PP is helpful.

\section{More Comparisons.}

Table~\ref{tab:ssb_new} and table\ref{tab:cch_new} shows the clustering accuracy of other methods adapted to solve the GCD task,
including the conventional clustering algorithm (k-means~\cite{macqueen1967some}), NCD methods (RankStats+~\cite{han2021autonovel} and UNO+~\cite{fini2021unified}), and method used to solve the open-world semi-supervised learning (ORCA~\cite{cao2021openworld}). From this table, we can see that though these methods take the category number as a prior, our proposed PNP still consistently outperforms these methods.

Table~\ref{tab:ssb_new} and table\ref{tab:cch_new} show the publicly available clustering accuracy of some methods on {\textbf{Oxford Pets}}~\cite{parkhi2012cats}. The Oxford Pets is a fine-grained dataset that consists of 3.6k instances from 37 classes.  Align with~\cite{rastegar2023learn,pu2023dynamic}, we sample 19 classes as the  ``Old'' classes ($\mathcal{Y}^l$) and and keep the rest as ``New'' ($\mathcal{Y}^u \textbackslash \mathcal{Y}^l$). Compared to DCCL~\cite{pu2023dynamic},  higher clustering accuracy on ``All'' classes is achieved by our proposed PNP demonstrating that PNP is also more effective than DCCL on the  Oxford Pets.

In methods that take the category number as a prior, SimGCD~\cite{wen2023parametric} is most similar to our proposed PNP, we reproduce SimGCD by eliminating the assumption of a known category number and report corresponding results in \cref{tab:ssb_new_new}. We can see that eliminating the prior drops the performance of SimGCD significantly. Moreover, under the original setting of GCD, \ie, the category number of unlabelled data is unknown, our proposed PNP consistently outperforms SimGCD.
